# Supplementary material for: Fast Algorithms for Minimum Homology Basis
Source: arXiv:2109.04567 source file (2024-06-07)
Supplement: Supplementary file 1 [file Appendix.tex]

\subsection{Implementation Details}
On a higher level, our implementation is based on \Cref{alg:hombasistwo}. 
Specifically, it differs from \Cref{alg:hombasistwo}, in its use of the specific  black box algorithms for minimum cycle basis and column rank profile. Below, we provide an overview of the main steps of the implementation.
\begin{algorithm}[H]
\caption{FastLoop : A Broad Overview}
\begin{algorithmic}[1]
\State Processing the input file: This includes populating the key data structures
\State Computing a min cycle basis. We use the  use the “Parallel Minimum Cycle Basis” library \cite{parmcb} to compute a minimum cycle basis of the $1$-skeleton on the input simplicial complex. It makes use of the Boost Library for storing the graph. There are multiple algorithms to choose from, with parallelized versions of the same. Parallelism is achieved through MPI  and Intel TBB library. The algorithms are based on the paper \cite{ImplMinCycBasis} by Michail and Melhorn.
\State We assemble the matrix $\newmatrix$ (boundary matrix prepended to the minimum cycle basis) see \ref{alg:hombasistwo}. Any suitable column reduction algorithm, that adds columns from left to right, can be used to compute the col rank profile. This matrix is sparse. A suitable implementation exploiting this sparsity property is the standard reduction algorithm in the PHAT library \cite{PHAT}, which we use for reducing the augmented matrix
\end{algorithmic}
\end{algorithm}

\begin{algorithm}[H]
\caption{FastLoop}\label{alg:fastloop}
\begin{algorithmic}[1]
\State Input : A file containing the 2-skeleton of the complex. see \ref{sec:ip-op-format}
\State Output: $\{\beta_1, minHomBasis\}$ see \ref{sec:ip-op-format}
\Procedure{FastLoop}{}
\State Process the input complex, populate $vertexList$, $triangles$, $vertexPairToEdgeNoMap$, $edgeNoToVertexPair$, $edgeNoToWeightMap$ see \ref{sec:ip-op-format}
\State Compute $graph$ see \ref{sec:ip-op-format}
\State $minCycleBasis \gets MINIMUM CYCLE BASIS(graph, vertexPairToEdgeNoMap)$ see \ref{alg:getMCB}
\State $\beta_1, minHomBasis \gets GET MIN HOMOLOGY BASIS(minCycleBasis, 
vertexPairToEdgeIndexMap, triangles, edgeNoToWeightMap)$ see \ref{alg:getMHB}
\State Return the minimum homology basis as a list of cycles as in \ref{sec:ip-op-format}, use $edgeNoToVertexPair$ to reverse map the $edgeNo$s in $minHomBasis$ to the desired output format
\EndProcedure
\end{algorithmic}
\end{algorithm}

\begin{algorithm}
\caption{GetMinimumCycleBasis} \label{alg:getMCB}
\begin{algorithmic}[1]
\vspace{1.5mm}
\State{Input: $graph$ represented as Boost Graph Data Structure, $vertexPairToEdgeIndexMap$: a C++ Map whose each key is a vertex-pair representing an edge in $graph$ and each value is the integer that edge is assigned in our enumeration of edges}\label{alg:getMCB_IP}
\State{Output: $cycles$: the cycles of a minimum cycle basis where each cycle is a list of edges. Each edge is represented as $edgeNo$}\label{alg:getMCB_OP}
\Procedure {Minimum Cycle Basis}{$graph$, $vertexPairToEdgeIndexMap$}
\State{
$mcbCyclesAsVertexPairList$ $\leftarrow$ parmcb::getmincyclebasis
}\Comment{A min cycle basis where each cycle is a list of edges, essentially vertex pairs in Boost Edge data format }
\Statex
\For{ $i$ from $1$ to $mcbCyclesAsVertexPairList.size()$}
\State $cycle$ $\leftarrow$  cycle at index $i$ of $mcbCyclesAsVertexPairList$

\State $edgesInCycle$ $\leftarrow$ \{\} \Comment{Initialized to an empty list}
\For{$j$ from $1$ to $cycle.size()$}
\State{
$vertexPair$ $\gets$ edge at index $j$ of $cycle$
}
\State{ Look up for corresponding $edgeNo$ for $vertexPair$ in $vertexPairToEdgeIndexMap$ and add it to $edgesInCycle$}
\EndFor
\State{Add $edgesInCycle$ to $cycles$}
\EndFor
\State return $cycles$
\EndProcedure
\end{algorithmic}
\end{algorithm}

\begin{algorithm}
\caption{Get Minimum Homology Basis} \label{alg:getMHB}
\begin{algorithmic}[1]
\vspace{1.5mm}
\State Input: $minCycleBasis$ the minimum cycle basis cycles in same format as in \algref{alg:getMCB}{alg:getMCB_OP}, $vertexPairToEdgeIndexMap$ as in \algref{alg:getMCB}{alg:getMCB_IP}, $triangles$: list of all faces, each face is $3$-tuple of its vertex indices, $edgeNoToWeightMap$: map whose each key-value pair is $edgeNo$ and corresponding edge weight
\State Output: $minHomBasis$, $\beta_1$
\Procedure {get Min Homology Basis}{$minCycleBasis$, $vertexPairToEdgeIndexMap$,
$triangles$,$edgeNoToWeightMap$
}
\State  $sortedMinCycleBasis \gets$ cycles of $minCycleBasis$ sorted by weight \Comment{Uses $edgeNoToWeightMap$ for sorting}
\Statex
\Comment{Prepare $\newmatrix$ as in \ref{alg:hombasistwo} }
\ForAll{$triangle$ in $triangles$} \Comment{$triangle$ is $3$-tuple of vertex indices}
\State $e_1, e_2, e_3 \gets$ $edgeNo$ of the $3$ edges of $triangle$ \Comment{Looks up $vertexPairToEdgeIndexMap$}
\State $columnVector \gets \{e_1, e_2, e_3\}$ in sorted order
\State Add $colVector$ to $\newmatrix$
\EndFor
\ForAll{$cycle$ in $sortedMinCycleBasis$}\Comment{$cycle$ is a list of $edgeNo$}
\State $columnVector \gets$ edges of $cycle$ in sorted order
\State Add $colVector$ to $\newmatrix$
\EndFor
\State Reduce $\newmatrix$, see \ref{alg:standardReduction}
\Statex
\Comment{Look for non-zero columns of $\newmatrix$ that correspond to cycles of the minimum cycle basis}

\State $\beta_1 \gets 0$
\State $minHomBasis \gets \{\}$
\For{$i = 1$ to $minCycleBasis.size()$}
\If{column $i + triangles.size()$ is non-zero}
\State $\beta_1 \gets \beta_1 + 1$
\State add $sortedMinCycleBasis[i]$ to $minHomBasis$
\EndIf
\EndFor
\State return $\{beta_1, minHomBasis\}$
\EndProcedure
\end{algorithmic}
\end{algorithm}

\subsection{PHAT Reduction}
PHAT {cite} is a library of matrix reduction algorithms for computing Barcodes in Persistent Homology. It implements a suite of algorithms in C++ for reducing the Boundary Matrix. {cite}. For our application we use Standard Reduction Algorithm for computing the column rank profile of the Prepended Matrix as the algorithm adds columns from left to right to perform the reduction {refer}. Our choice is also motivated by the fact that PHAT's implementation exploits the sparsity of the Prepended Matrix, besides being a simple algorithm in itself. We reproduce the Standard Reduction Algorithm here for convenience, see \ref{alg:standardReduction}
